# Supplementary material for: Distributionally Robust Ground Delay Programs with Learning-Driven Airport Capacity Predictions
Source: arXiv:2402.11415 source file (2024-02-18)
Supplement: Supplementary file 1 [file appendix1.tex]

\thispagestyle{firststyle}
% \clearpage

% \documentclass{article}
% \usepackage{graphicx}
% \usepackage{subcaption}

% \documentclass[conference,10pt]{../IEEEtran_ICRATmod}

% \IEEEoverridecommandlockouts
% \overrideIEEEmargins

% \oddsidemargin=-0.5in
% \evensidemargin=-0.5in
% \textwidth=7.5in
% \textheight=8.7in
% \columnsep=0.5in

% \usepackage[numbers]{natbib}
% % \usepackage{subfig}
% \usepackage{subfigure}
% \usepackage{graphics} % for pdf, bitmapped graphics files
% \usepackage{epsfig} % for postscript graphics files
% %\usepackage{mathptmx} % assumes new font selection scheme installed
% \usepackage{times} % assumes new font selection scheme installed
% \usepackage{amsmath} % assumes amsmath package installed
% \usepackage{amssymb}  % assumes amsmath package installed
% \usepackage{amsthm}
% \usepackage{amsfonts}
% \usepackage{mathtools}
% \usepackage{multirow} % allows mutli-row and multi-column tables
% \usepackage{rotating} % allows for sideways text in tables
% \usepackage{graphicx}
% \usepackage{float}
% \usepackage{flushend}
% %\usepackage{xcolor}
% \usepackage[table,xcdraw]{xcolor}
% \usepackage{csquotes}
% \usepackage{bm}
% \usepackage{relsize}
% \usepackage{epspdfconversion}
% \usepackage{colortbl}
% \usepackage{lipsum}
% \usepackage[mathscr]{eucal}
% \usepackage{fancyhdr}


% \begin{document}

\section*{Appendix I: Deriving actual capacities from throughput}  \label{sec:appendix1}

% As mentioned in Section~\ref{sec:methodology}, real-time capacity need to estimated from throughput based on the rule shown in equations~\ref{eq: capacity_estimation}. Table~\ref{tab:airport_coefficient_tau} summaries the detailed selection of $\tau$ for each airport.

% Based on actual airport arrival and departure throughput, we derive estimates of the actual capacity by first noting that the throughput at time $t$ (observable) is the minimum of the demand at time $t$ (observable) and the actual capacity at time $t$ (unobservable, to be estimated). 

% Deriving real-time airport capacity directly from historical records is challenging. 


% We derive estimates of the actual capacity from historical records of airport arrival and departure throughput directly. However, it is challenging that the throughput at time $t$ (observable) typically are underestimations of actual capacity at time $t$ (unobservable, to be estimated), particularly during not busy time periods. Thus, we need to select the peak operation time slices, when throughput approaches maximum capacity, making them as good indicators for large airports' capacity.

% We derive estimates of actual airport capacity directly from historical records of arrivals and departures. However, a significant challenge is that the observable throughput at time $t$ often underestimates the actual, yet unobservable, capacity at the same time, especially during off-peak periods. Therefore, our approach focuses on selecting slices of peak operational times. During these periods, throughput typically reaches its maximum, providing a more accurate indicator of capacity for large airports.

% Our approach utilizes two specific rules to select the most representative time slices where capacity aligns closely with actual AARs and ADRs, as shown in Equation~\ref{eq: capacity_estimation}. Rule 1 targets time periods where demand significantly exceeds throughput, useful in identifying mismatched demand-throughput scenarios. However, this rule may not always capture peak hours due to delay propagation effects. In contrast, Rule 2 focuses on periods of extreme delay, indicative of less initial demand but high operational intensity due to delay recovery. This rule highlights the impact of delay propagation on capacity estimation.

% Both rules are rigorously applied to arrival and departure data, selecting time slices that satisfy the following condition for capacity representation:

We estimate actual airport capacity using historical arrival and departure data. A key challenge in this process is that the observable throughput at a given time $t$ tends to underestimate the actual, yet unobservable, capacity, particularly during off-peak periods. To address this, our method concentrates on peak operational times when throughput generally reaches its maximum, thus offering a more reliable measure of large airports' capacity.

To identify the most representative time slices for capacity estimation, we employ two rules as defined in Equation~\ref{eq:capacity_estimation}. Rule 1 is applied to periods where there is a significant excess of demand over throughput, aiding in the identification of scenarios where demand and throughput are mismatched due to the capacity limitation. We choose a threshold $\tau=3$ to balance the need for better filtering of extremes and reducing data sparsity. However, Rule 1 may not consistently pinpoint peak hours due to delay propagation effects, which can lead to high operational activity following initially low demand. On the other hand, Rule 2 targets periods with extreme delays (i.e., delay more than 30 mins), while discounting anomalies caused by one single delayed flights. Yet, this rule alone might overlook not-that-extreme peak periods with less delayed operations but actual capacity constraints. Therefore, we combine these rules to select periods where throughput accurately reflects capacity.

Both rules are stringently applied to arrival and departure data, selecting time slices where meet the conditions in Equation~\ref{eq:capacity_estimation}, outlined as follows:

\begin{equation}
\label{eq:capacity_estimation}
    \widehat{\text{capacity}}_t = \text{throughput}_t \iff \text{(Rule 1)} \lor \text{(Rule 2)}
\end{equation}
\begin{align*}
    & \text{ Rule 1:} \quad \text{demand}_t \geq \text{throughput}_t + 3 \\
    & \text{ Rule 2:} \quad \left(\text{Avg delay}_t > 30\right) \land \left(\text{No. of delayed flights}_t > 1 \right)
\end{align*}

To better illustrate the effect of capacity estimation deriving from throughput according to the rules, we take the LAX airport (the same as result analysis) as case study. Fig.~\ref{fig:lax_traffic_ranking_raw} depicts the LAX airport's hourly throughput over a year ranking from busiest to idlest hour. During the morning around 8am-12am, the airport's arrival throughput reaches an apex, representing nearly 100 hours of exceptionally high traffic over the year—approximately top 10\% of the total dataset. For departure throughput, the afternoon will have a busier operations. Conversely, the least busy hours, are identified typically during 0-6am, where both of the arrival and departure throughput substantially falls below the airport's capacity.

%\begin{figure}[htp]
%    \centering
%    \includegraphics[width=0.45\textwidth]{ICRAT2024_predictDRO/figures/capacity_prediction_figure/ORD_traffic_ranking.png}
%    \caption{Hourly throughput ranking in 2019 for ORD Airport.}
%    \label{fig:ord_traffic_ranking_raw}
%\end{figure}

\begin{figure}[htp]
    \centering
    \includegraphics[width=0.45\textwidth]{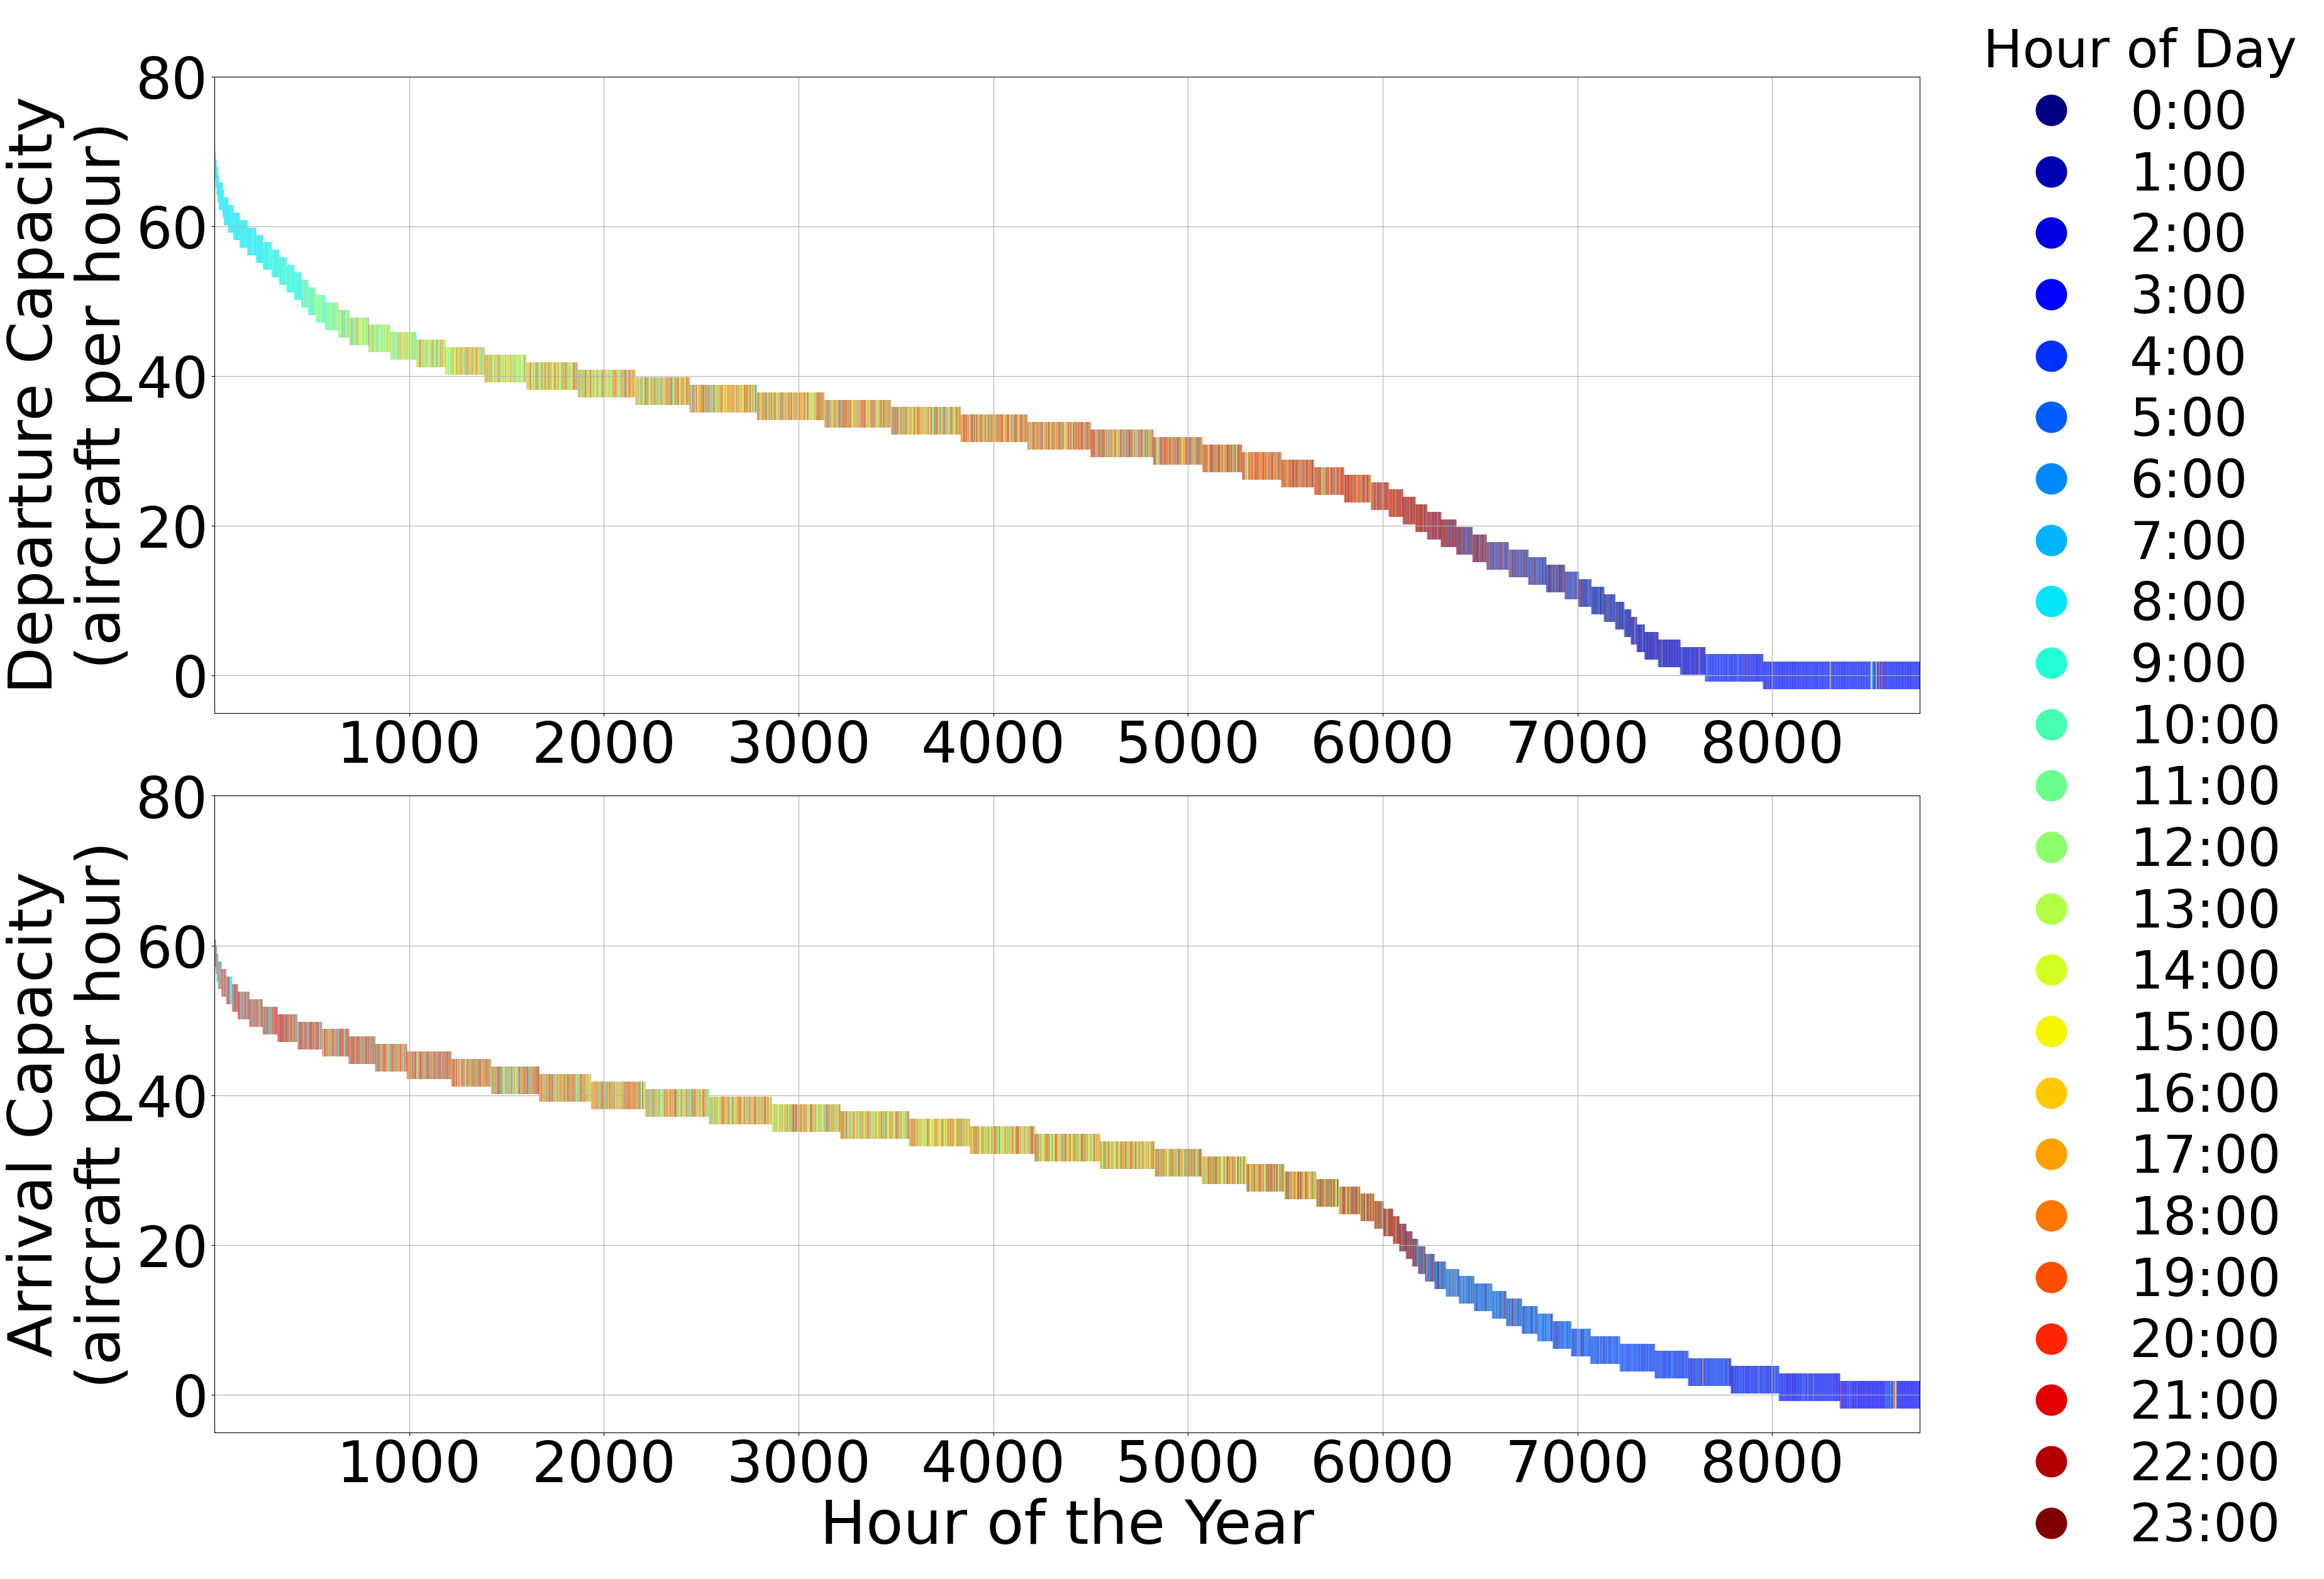}
    \caption{Hourly throughput ranking in 2019 for LAX Airport.}
    \label{fig:lax_traffic_ranking_raw}
\end{figure}

However, after the rules selecting the time slices to estimate capacity from throughput, as shown in Fig.~\ref{fig:lax_capacity_rankings}, most of the data from the early morning hours on the right of the original Fig.~\ref{fig:lax_capacity_ranking_combined_ruled} are mostly filtered out. Specifically, the morning hours are more selecting by Rule 1 in Eq.~\ref{eq:capacity_estimation}, illustrated in Fig.~\ref{fig:lax_capacity_ranking_tau_ruled}. While Rule 2 mainly focus on the afternoon and evening time slices' operations as shown in Fig.~\ref{fig:lax_capacity_ranking_delay_ruled}. This approach for selecting the capacity estimation time slices thus confirms our objective: filtering out extreme values and periods of low busy activity, using the remaining throughput data to estimate airport capacity. 

\begin{figure}[htbp]
\centering
    \subfloat[\label{fig:lax_capacity_ranking_combined_ruled} Time slices selected by Eq.~\ref{eq:capacity_estimation}.]{\includegraphics[width=0.45\textwidth]{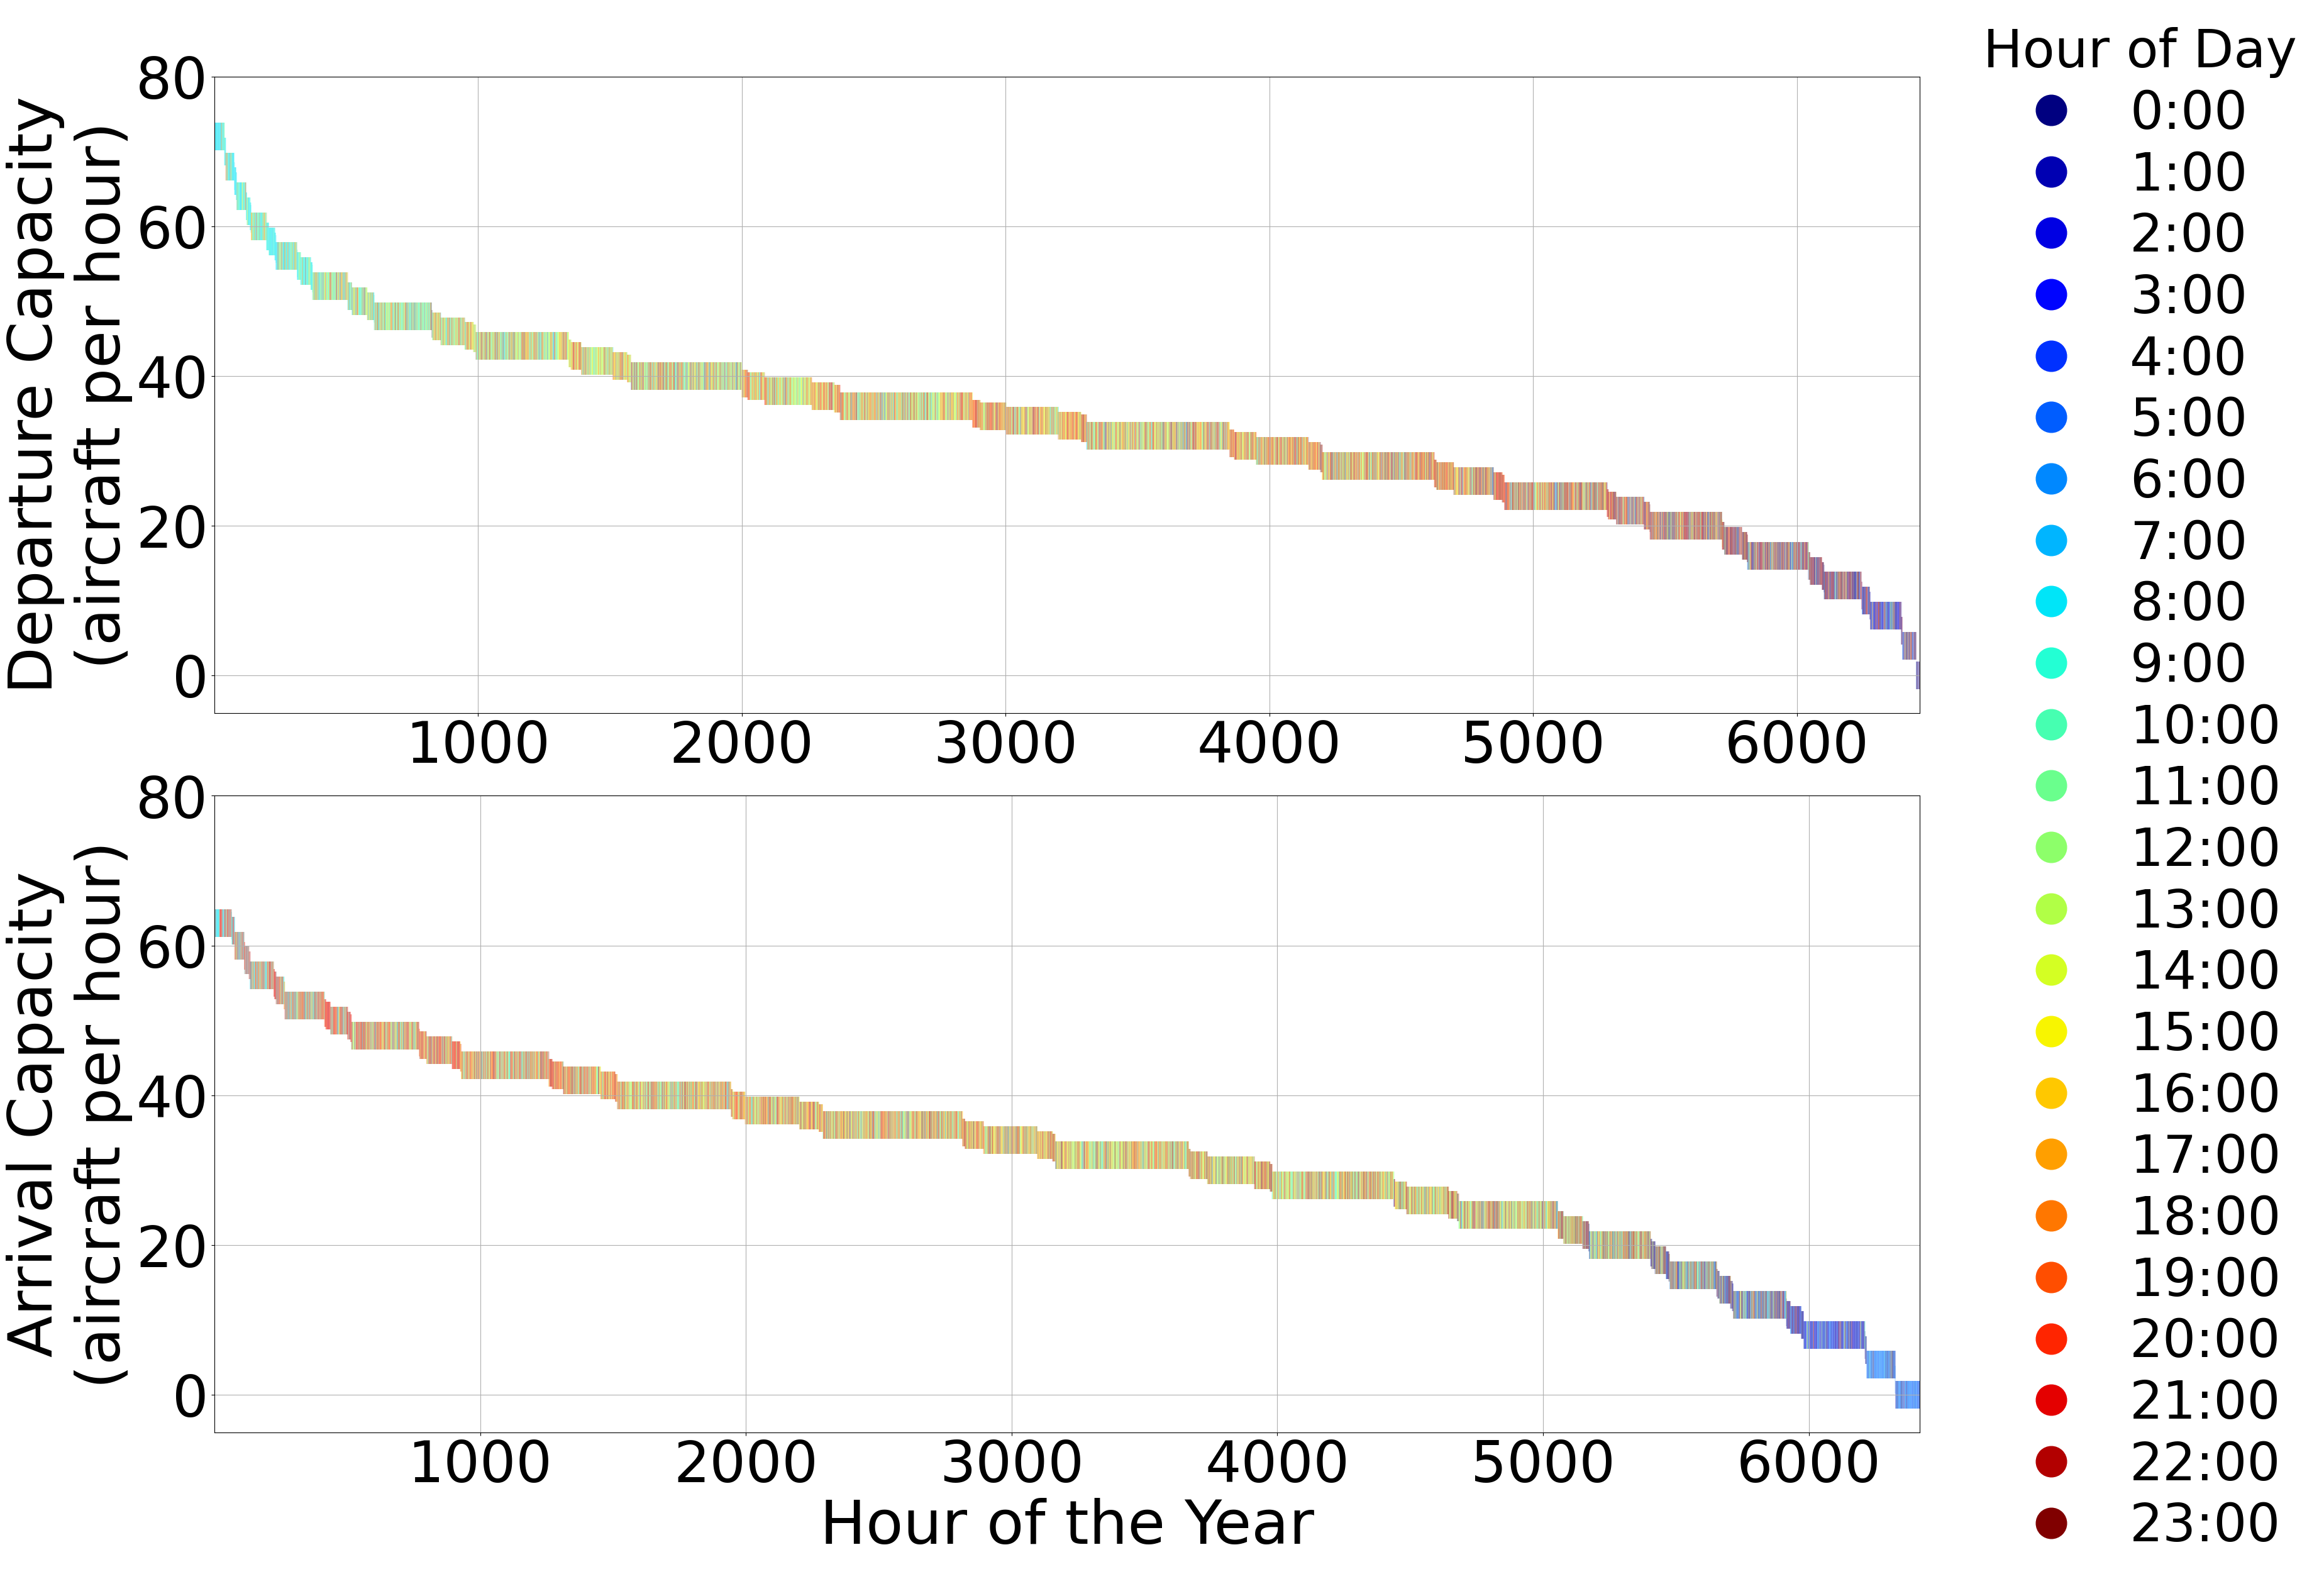}}
    \vfill
    \subfloat[\label{fig:lax_capacity_ranking_tau_ruled} Time slices selected by Rule 1 only in Eq.~\ref{eq:capacity_estimation}.]{\includegraphics[width=0.45\textwidth]{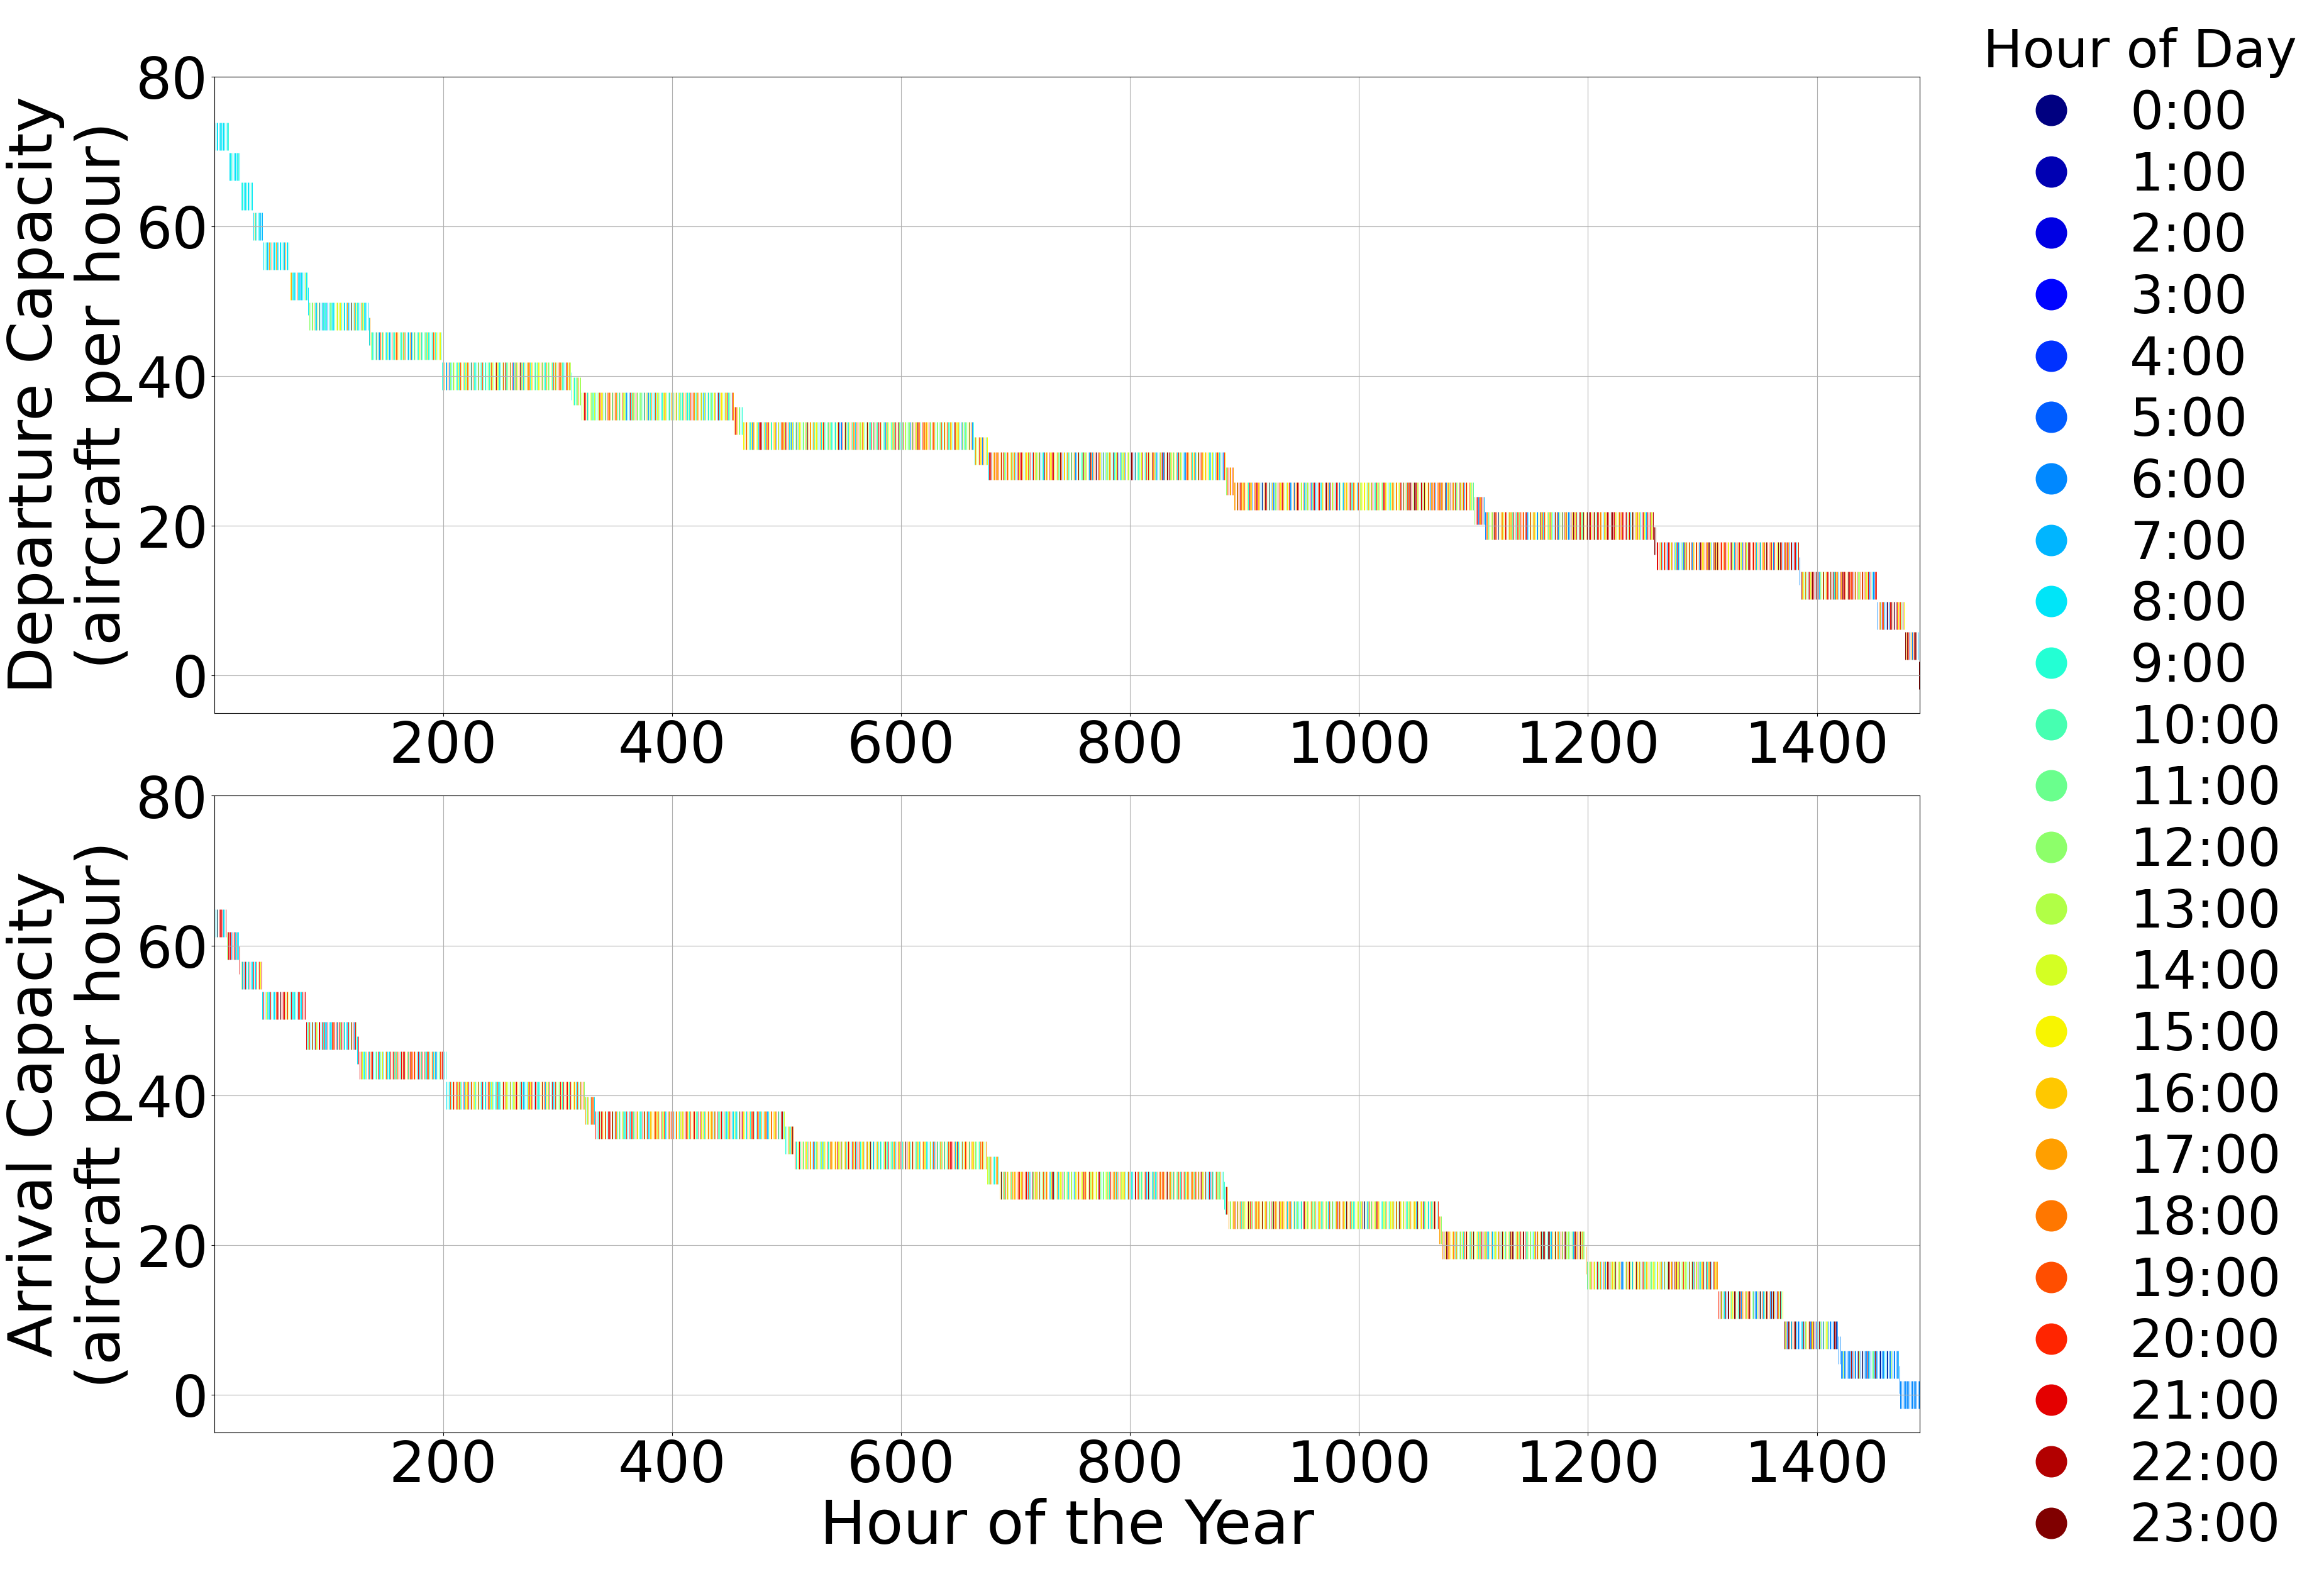}}
    \vfill
    \subfloat[\label{fig:lax_capacity_ranking_delay_ruled} Time slices selected by Rule 2 only in Eq.~\ref{eq:capacity_estimation}.]{\includegraphics[width=0.45\textwidth]{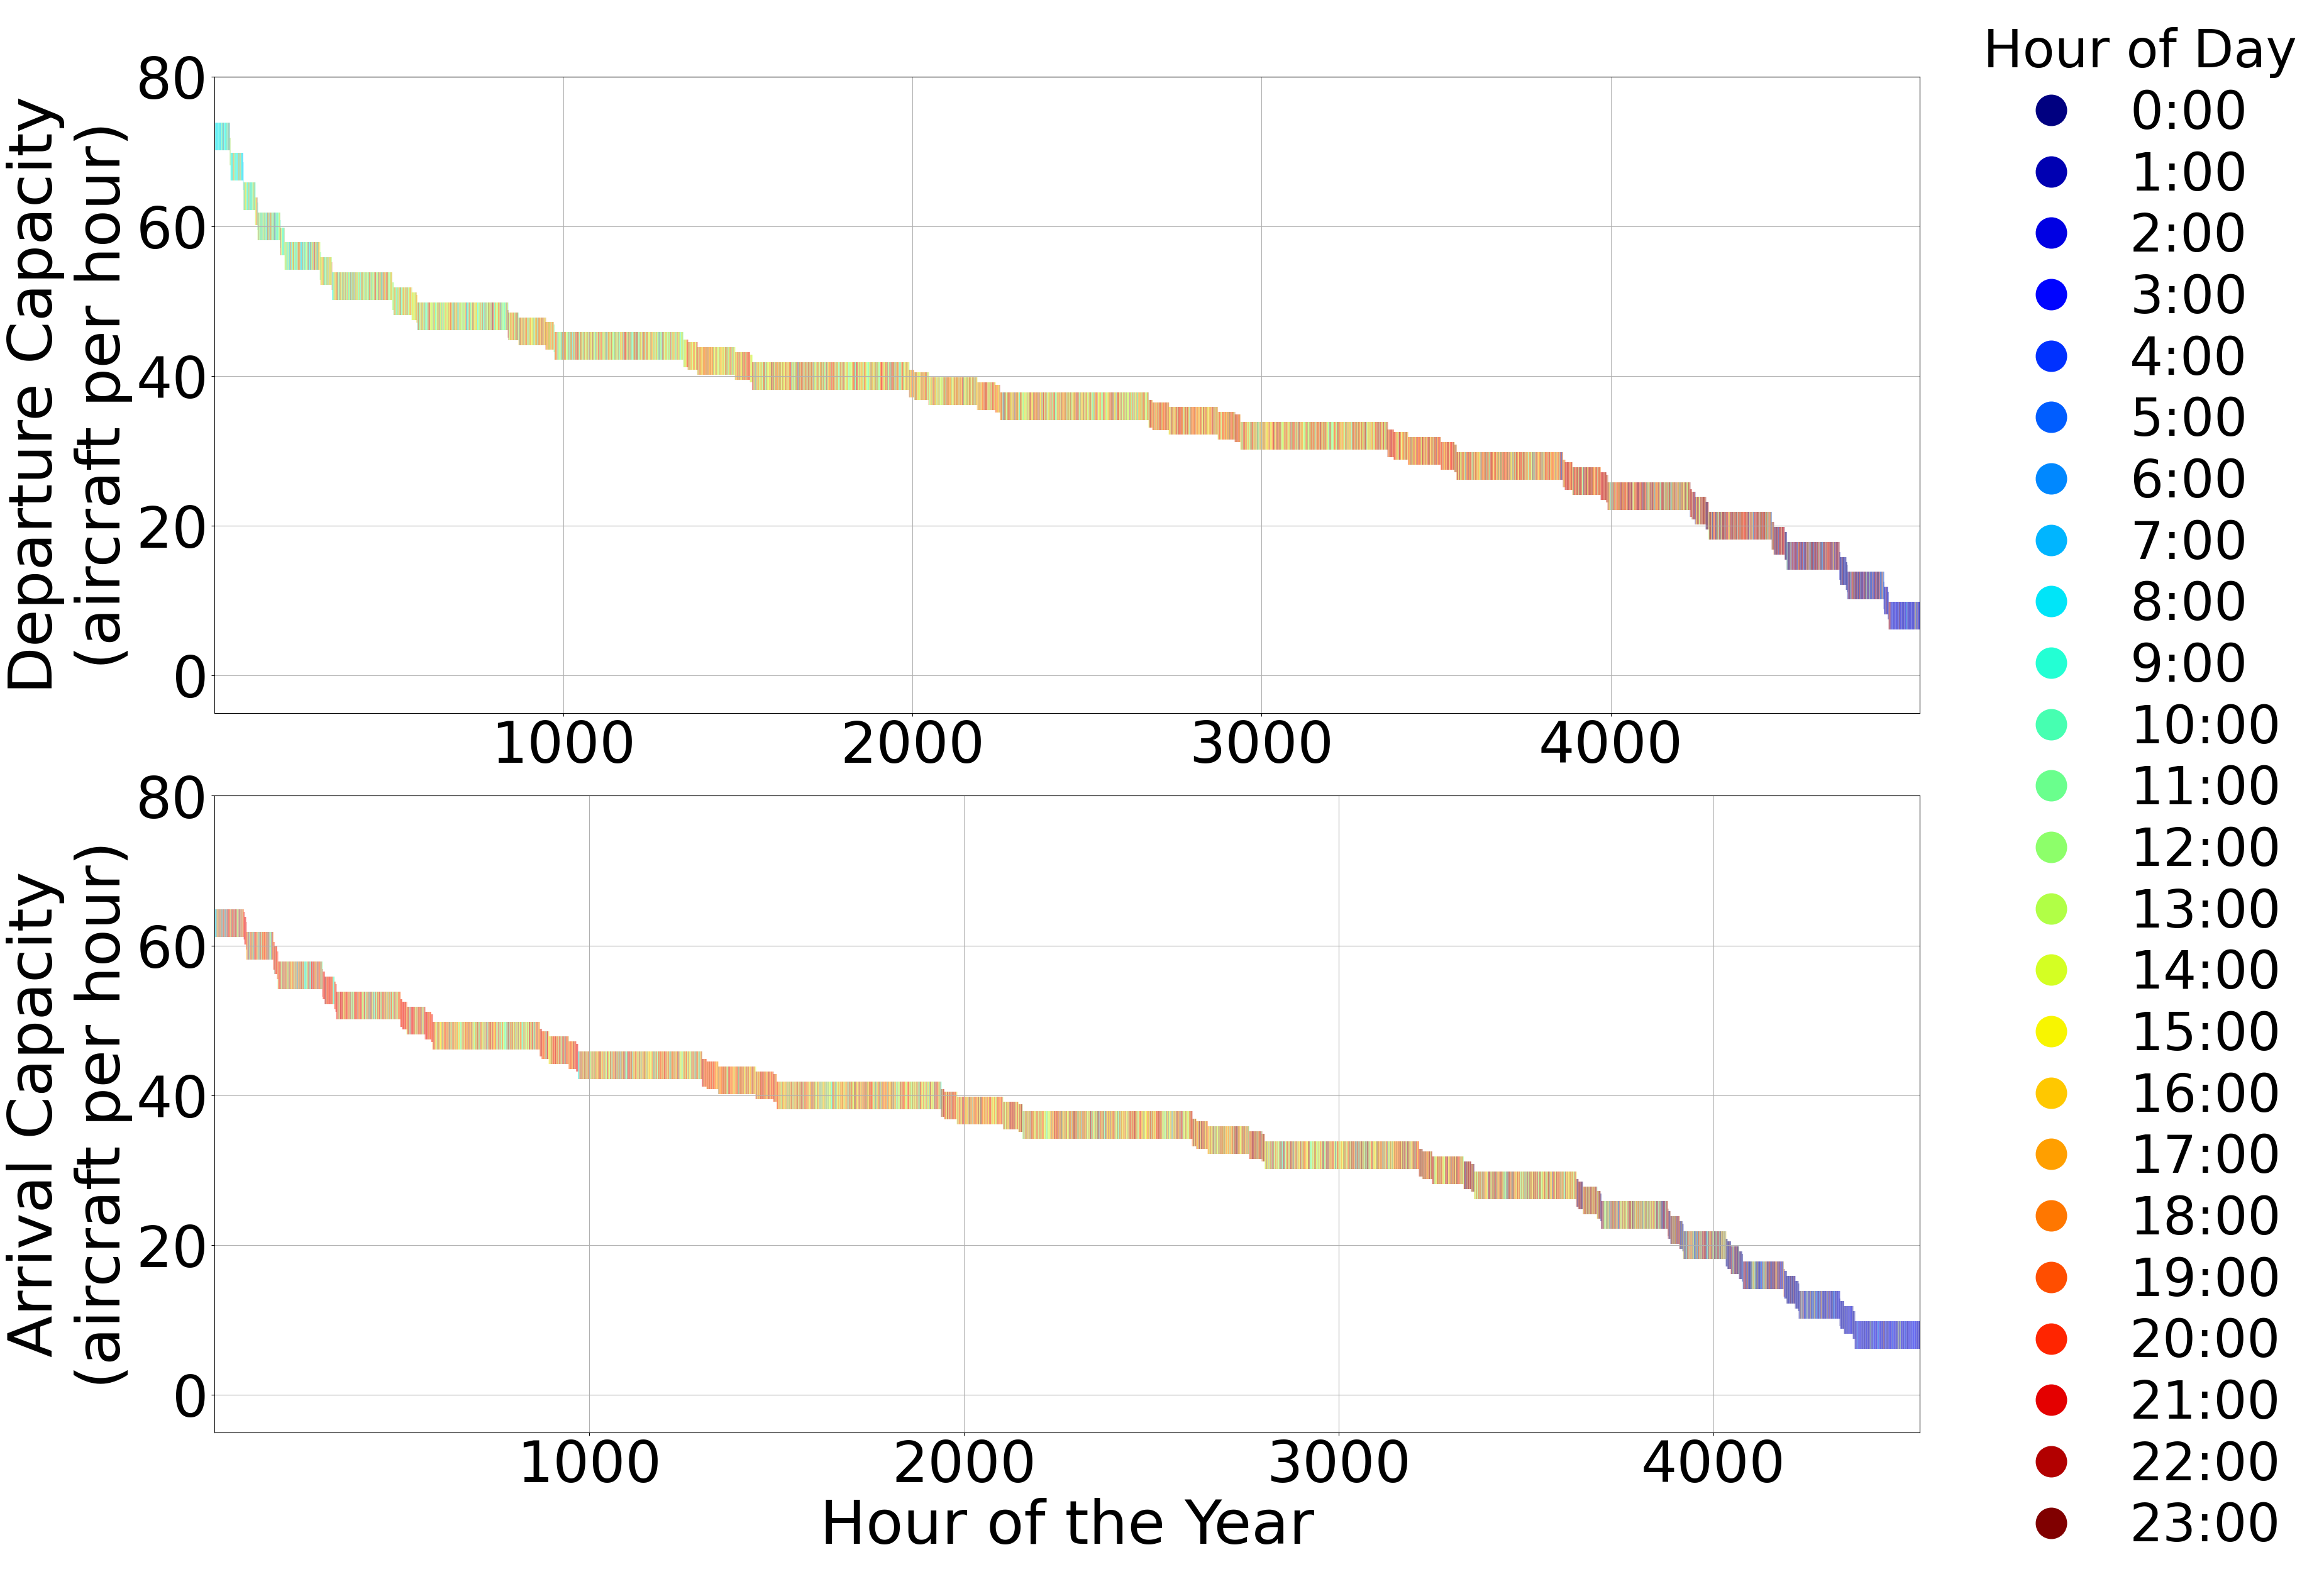}}
    \vfill
\caption{Comparison of hourly throughput rankings of the different time slices selected for LAX capacity estimation.}\label{fig:lax_capacity_rankings}
\end{figure}

% \begin{figure}[htp]
%     \centering
%     \includegraphics[width=0.45\textwidth]{ICRAT2024_predictDRO/figures/capacity_prediction_figure/LAX_capacity_ranking_tau.png}
%     \caption{Comparison of hourly throughput rankings of the different time slices selected by Rule 1 for LAX capacity estimation.}
%     \label{fig:ord_traffic_ranking_raw}
% \end{figure}



% \begin{figure}[htp]
%     \centering
%     \includegraphics[width=0.45\textwidth]{ICRAT2024_predictDRO/figures/capacity_prediction_figure/LAX_capacity_ranking_delay.png}
%     \caption{Comparison of hourly throughput rankings of the different time slices selected by Rule 2 for LAX capacity estimation.}
%     \label{fig:ord_traffic_ranking_raw}
% \end{figure}

% \begin{figure}[htp]
%     \centering
%     \includegraphics[width=0.45\textwidth]{ICRAT2024_predictDRO/figures/capacity_prediction_figure/LAX_capacity_ranking_combined.png}
%     \caption{Comparison of hourly throughput rankings of the different time slices selected by Rule 1 \& 2 for LAX capacity estimation.}
%     \label{fig:ord_traffic_ranking_raw}
% \end{figure}

% \end{document}




% The reason of AARs or ADRs cannot reflect the true capacity is that the AARs or ADRs always is an underestimates of the capacity, when the airport is in busy operation hours, the throughputs will close to the capacity which can be good candidates to estimate the airport capacity for large airports.

% As shown in theory, the $\text{throughput}_t = \min\{\text{demand}_t, \text{capacity}_t\}.$ thus rule 1 is applied to seclect the time period with The Rule 1 only focus on the demand-throughput unmatched time slices. But it is noted that with the delay propogation, the time period will not stand to select the busy hours. 

% while Rule 2 mainly focus on the delay period with extreme delay situations, which show the delay propagation period, with less demand in advance but have to operate as busy for the hours. 

% These two rules are strictly applied to the arrival and departure, and only the time slices with equation \ref{eq:capacity_estimation} stands for both arrival and departure are selected to represent the capacity.


% \begin{equation}\lable{eq:capacity_estimation}
%     \widehat{\text{capacity}}_t = \text{throughput}_t \iff \text{(Rule 1)} \lor \text{(Rule 2)}
% \end{equation}
% \begin{align*}
%     \text{where}
%     & \text{ Rule 1:} \quad \text{demand}_t \geq \text{throughput}_t + 3 \\
%     & \text{ Rule 2:} \quad \left(\text{Avg delay}_t > 30\right) \land \left(\text{No. of delayed flights}_t > 1 \right)
% \end{align*}



% % \text{where:}
% \begin{itemize}
%     \item \text{Rule 1 is satisfied if:} \quad \text{demand}_t \geq \text{throughput}_t + 3.
%     \item \text{Rule 2 is satisfied if both:} \quad \text{Avg delay}_t > 30 \quad \text{and} \quad \text{No. of flights}_t > 1.
% \end{itemize}



% \begin{equation}
%     \widehat{\text{capacity}}_t = \text{throughput}_t \iff 
%     \begin{cases}
%         \text{demand}_t \geq \text{throughput}_t + 3, & \text{(Rule 1)} \\
%         \text{Avg delay}_t > 30 \text{ AND } \text{No. of flights}_t > 1 & \text{(Rule 2)}
%     \end{cases}
% \end{equation}

% \end{document}


% \begin{equation}
%     \widehat{\text{capacity}}_t = \text{throughput}_t \quad \text{if and only if} \quad \left( \text{Condition of Rule 1} \quad \text{or} \quad \text{Condition of Rule 2} \right) \quad \text{is met},
% \end{equation}
% \text{where:}
% \begin{align*}
%     &\text{Condition of Rule 1 is met if:} \\
%     &\quad \text{demand}_t \geq \text{throughput}_t + 3. \\
%     &\text{Condition of Rule 2 is met if both of the following are true:} \\
%     &\quad \text{Avg delay}_t > 30 \quad \text{minutes}, \\
%     &\quad \text{No. of flights}_t > 1.
% \end{align*}

% \begin{equation}
%     \widehat{\text{capacity}}_t = \text{throughput}_t \iff 
%     \left[ \text{demand}_t \geq \text{throughput}_t + 3 \right] 
%     \text{ OR }
%     \left[ \text{Avg delay}_t > 30 \text{ AND } \text{No. of flights}_t > 1 \right].
% \end{equation}



% Rule 1 


% Rule 1: 
% \begin{equation}\label{eq: capacity_estimation}
%     \begin{aligned}
%     \widehat{\text{capacity}}_t = \text{throughput}_t \iff  
%     & \text{demand}_t \geq \text{throughput}_t + 3
%     \\ 
%     \cup 
%     \\ 
%     & \left\{  
%     \begin{aligned}
%      \text{Avg delay}_t > 30 \\
%      \text{No. of flights}_t > 1
%     \end{aligned}
%     \right.
%     \end{aligned}
% \end{equation}

% Rule 2: 
% \begin{equation}
%     \widehat{\text{capacity}}_t = \text{throughput}_t \iff 
%     \left\{  
%     \begin{aligned}
%      \text{Avg delay}_t > 30 \\
%      \text{No. of delayed flights}_t > 1
%     \end{aligned}
%     \right.,
% \end{equation}
% where $\hat{\text{capacity}}_t$ denotes the estimated capacity at time slice $t$. $\text{throughput}_t$ denotes the throughput at time slice $t$.\par



% Based on actual airport arrival and departure throughput, we derive estimates of the actual capacity by first noting that the throughput at time $t$ (observable) is the minimum of the demand at time $t$ (observable) and the actual capacity at time $t$ (unobservable, to be estimated). We estimate the capacity at time $t$ to be equal to the throughput at time $t$, while enforcing that demand at time $t$ must be greater than or equal to the observed throughput at time $t$ plus an integer threshold $\tau$. 

% The critical step for our estimation process relies on selecting $\tau$ to filter out historical throughput that may be extreme under- or over-estimations of the actual, unobservable capacity. If $\tau$ is too small, the extremes may not be filtered out. If $\tau$ is too large, we are left with a sparse historical data set. Note that we tune a different $\tau$ for each airport due to differing operational characteristics, and because we construct a prediction model for each airport. Due to page limitations, we refer readers to Appendix \ref{sec:appendix1} for details on selecting $\tau$.

% Selecting the most typical time slices from the throughput at each 15-minute interval according to defined rules. 

% Specifically, as shown in Equations~\ref{eq: capacity_estimation}, we suppose that the throughput at time $t$ can be represented as 
% \begin{equation}
%     \text{throughput}_t = \min\{\text{demand}_t, \text{capacity}_t\}. 
% \end{equation}
% Thus we have

% Rule 1:  
% \begin{equation}\label{eq: capacity_estimation}
%     \begin{aligned}
%     \widehat{\text{capacity}}_t = \text{throughput}_t \iff  
%     & \text{demand}_t \geq \text{throughput}_t + 3
%     \\ 
%     \cup 
%     \\ 
%     & \left\{  
%     \begin{aligned}
%      \text{Avg delay}_t > 30 \\
%      \text{No. of flights}_t > 1
%     \end{aligned}
%     \right.
%     \end{aligned}
% \end{equation}

% Rule 2: 
% \begin{equation}
%     \widehat{\text{capacity}}_t = \text{throughput}_t \iff 
%     \left\{  
%     \begin{aligned}
%      \text{Avg delay}_t > 30 \\
%      \text{No. of delayed flights}_t > 1
%     \end{aligned}
%     \right.,
% \end{equation}
% where $\hat{\text{capacity}}_t$ denotes the estimated capacity at time slice $t$. $\text{throughput}_t$ denotes the throughput at time slice $t$.\par


% We filter the dataset through this definition and control the size of the dataset after estimating capacity using $\tau$. 



% this $\tau$ parameter is airport-specific, as we


% The larger the $\tau$, the smaller the filtered dataset and the more possible estimated capacity. Therefore, selecting an appropriate $\tau$ is a focus. 

% Since each model is trained on a specific airport's dataset, the choice of $\tau$ needs to be based on the parameters of each airport model. Based on these $\tau$ determined separately for each airport's arrival and departure capacity estimates, we filter out time samples when operations are not congested and retain time samples during busy periods, and approximate the real-time capacity to the actual throughput for that time step. 

% However, it is also noted that using this rule~\ref{eq: capacity_estimation}, capacity is always underestimated as throughput, and busy periods in the evening due to delay propagation are also eliminated. Detailed procedures of coefficient selection is represented in Appendix~\ref{sec:appendix1}. \par







% \begin{table}[htp]
%     \centering
%     \resizebox{0.47\textwidth}{!}{
%     % \footnotesize
%     \begin{tabular}{c|c|c|c|c}
%         \hline
%         \hline
%         Airport & \multicolumn{2}{c|}{Arrival Capacity} & \multicolumn{2}{c}{Departure Capacity} \\ \cline{2-5}
%         & Coefficient $\tau$ & \multirow{2}{*}{Data Left} & Coefficient $\tau$ & \multirow{2}{*}{Data Left} \\
%         & & \multirow{2}{*}{Percentage (\%)} & & \multirow{2}{*}{Percentage (\%)} \\ 
%         & & & & \\ \hline
%         ATL & 2 & 29.00\% & 1 & 34.88\% \\
%         BOS & 2 & 26.12\% & 2 & 23.84\% \\
%         BWI & 2 & 21.59\% & 1 & 30.89\% \\
%         CLT & 2 & 25.44\% & 1 & 31.53\% \\
%         DCA & 2 & 23.13\% & 2 & 23.31\% \\
%         DEN & 1 & 33.35\% & 1 & 34.85\% \\
%         DFW & 1 & 34.77\% & 1 & 32.02\% \\
%         DTW & 1 & 31.06\% & 1 & 28.74\% \\
%         EWR & 2 & 27.06\% & 2 & 26.91\% \\
%         FLL & 1 & 35.43\% & 1 & 31.76\% \\
%         HNL & 1 & 27.13\% & 1 & 26.32\% \\
%         IAD & 1 & 23.99\% & 1 & 24.08\% \\
%         IAH & 1 & 28.68\% & 1 & 28.68\% \\
%         JFK & 2 & 25.12\% & 1 & 33.14\% \\
%         LAS & 2 & 23.50\% & 2 & 23.67\% \\
%         LAX & 2 & 28.15\% & 1 & 37.38\% \\
%         LGA & 2 & 25.26\% & 2 & 25.76\% \\
%         MCO & 2 & 24.09\% & 2 & 21.63\% \\
%         MDW & 2 & 18.99\% & 1 & 29.95\% \\
%         MEM & 1 & 22.76\% & 1 & 20.53\% \\
%         MIA & 1 & 32.14\% & 1 & 28.58\% \\
%         MSP & 1 & 32.41\% & 1 & 30.05\% \\
%         ORD & 2 & 32.35\% & 1 & 36.49\% \\
%         PHL & 2 & 23.69\% & 1 & 31.84\% \\
%         PHX & 2 & 24.04\% & 1 & 34.65\% \\
%         SAN & 1 & 29.79\% & 1 & 29.12\% \\
%         SEA & 2 & 25.55\% & 1 & 34.73\% \\
%         SFO & 2 & 26.02\% & 2 & 25.78\% \\
%         SLC & 1 & 29.04\% & 1 & 29.50\% \\
%         TPA & 2 & 16.96\% & 1 & 28.16\% \\
%         \hline
%         \hline
%     \end{tabular}}
%     \caption{Summary of coefficient $\tau$ selection and left percentage for each airport's arrival and departure.}
%     \label{tab:airport_coefficient_tau}
% \end{table}


%\begin{table}[htp]
%    \centering
%    \resizebox{0.45\textwidth}{!}{
%    % \footnotesize
%    \begin{tabular}{c|c|c|c|c}
%        \hline
%        \hline
%        Airport & \multicolumn{2}{c|}{Arrival Capacity} & \multicolumn{2}{c}%{Departure Capacity} \\ \cline{2-5}
%        & Coefficient $\tau$ & \multirow{2}{*}{Data Left} & Coefficient $\tau$ & \multirow{2}{*}{Data Left} \\
%        & & \multirow{2}{*}{Percentage (\%)} & & \multirow{2}{*}{Percentage (\%)} \\ 
%        & & & & \\ \hline
%        ATL & 3 & 29.00\% & 1 & 34.88\% \\
%        BOS & 3 & 26.12\% & 2 & 23.84\% \\
%        BWI & 3 & 21.59\% & 1 & 30.89\% \\
%        CLT & 3 & 25.44\% & 1 & 31.53\% \\
%        DCA & 3 & 23.13\% & 2 & 23.31\% \\
%        DEN & 3 & 33.35\% & 1 & 34.85\% \\
%        DFW & 3 & 34.77\% & 1 & 32.02\% \\
%        DTW & 3 & 31.06\% & 1 & 28.74\% \\
%        EWR & 2 & 27.06\% & 2 & 26.91\% \\
%        FLL & 1 & 35.43\% & 1 & 31.76\% \\
%        HNL & 1 & 27.13\% & 1 & 26.32\% \\
%        IAD & 1 & 23.99\% & 1 & 24.08\% \\
%        IAH & 1 & 28.68\% & 1 & 28.68\% \\
%        JFK & 2 & 25.12\% & 1 & 33.14\% \\
%        LAS & 2 & 23.50\% & 2 & 23.67\% \\
%        LAX & 2 & 28.15\% & 1 & 37.38\% \\
%        LGA & 2 & 25.26\% & 2 & 25.76\% \\
%        MCO & 2 & 24.09\% & 2 & 21.63\% \\
%        MDW & 2 & 18.99\% & 1 & 29.95\% \\
%        MEM & 1 & 22.76\% & 1 & 20.53\% \\
%        MIA & 1 & 32.14\% & 1 & 28.58\% \\
%        MSP & 1 & 32.41\% & 1 & 30.05\% \\
%        ORD & 2 & 32.35\% & 1 & 36.49\% \\
%        PHL & 2 & 23.69\% & 1 & 31.84\% \\
%        PHX & 2 & 24.04\% & 1 & 34.65\% \\
%        SAN & 1 & 29.79\% & 1 & 29.12\% \\
%        SEA & 2 & 25.55\% & 1 & 34.73\% \\
%        SFO & 2 & 26.02\% & 2 & 25.78\% \\
%        SLC & 1 & 29.04\% & 1 & 29.50\% \\
%        TPA & 2 & 16.96\% & 1 & 28.16\% \\
%        \hline
%        \hline
%    \end{tabular}}
%    \caption{Summary of left percentage of selection $\tau=3$ for each airport's arrival and departure.}
%    \label{tab:airport_coefficient_tau}
%\end{table}

% To better illustrate the effect of capacity estimation from throughput according to the rule ~\ref{eq: capacity_estimation}, we take the ORD airport as case study. Fig.~\ref{fig:ord_traffic_ranking_raw} depicts the ORD airport's hourly throughput over a year ranking from busiest to idlest hour. Notably, during the 10am-12am, the airport's throughput reaches an apex, representing nearly 100 hours of exceptionally high traffic over the year—approximately 1\% of the total dataset. During these periods, the airport's throughput significantly exceeds its maximum capacity. Conversely, the chart also identifies the least busy hours, typically from 0-6am, where the throughput substantially falls below the airport's capacity. The purpose of this initial analysis is to inform our capacity estimation process. 

% However, after the rule selecting the time slices to estimate capacity from throughput, as shown in Fig.~\ref{fig:ord_traffic_ranking_tau_ruled}, the most extreme values on the left of the original Fig.~\ref{fig:ord_traffic_ranking_raw} are filtered out. Simultaneously, most of the data from the early morning hours on the right are also filtered out, while data from other time periods effectively estimate the airport capacity. This approach for selecting the capacity estimation coefficient thus achieves our objective: filtering out extreme values and periods of low busy activity, using the remaining throughput data to estimate airport capacity. This analysis confirms the selection of $\tau$ in the capacity estimation.














% In preparation for data analysis, we first ranked the airport's hourly throughput from highest to lowest and normalized these values to create a traffic ranking chart, as depicted in Figure \ref{fig:ord_traffic_ranking}. This chart, with color coding to delineate different time intervals, reveals a noteworthy pattern. Specifically,

% during the 10am-12am, the airport's throughput reaches an apex, representing nearly 100 hours of exceptionally high traffic over the year—approximately 1\% of the total dataset. During these periods, the airport's throughput significantly exceeds its maximum capacity. Conversely, the chart also identifies the least busy hours, typically from 0-6am, where the throughput substantially falls below the airport's capacity. The purpose of this initial analysis is to inform our capacity estimation process. In the capacity estimation section, following rule ~\ref{eq: capacity_estimation}, we obtain five filtered datasets. It is evident that a larger $\tau$ results in a reduced samples of data, which  leads to more accurate estimations. Balancing the samples of data with the accuracy of estimation is a crucial consideration. In this part, for each model, we apply the criterion that
% \begin{equation}\label{eq: sample_parameter}
%     samples>5 \times parameter,
% \end{equation}

% and choose the largest $\tau$ that meets this rule, where 'parameters' refers to the parameters of each model. Taking ORD airport as an example, as illustrated in Figure \ref{fig:ord_capacity_ranking}, the data post-estimation sees the most extreme values on the left of the original data filtered out. Simultaneously, most of the data from the early morning hours on the right are also filtered out, while data from other time periods effectively estimate the airport capacity. This approach for selecting the capacity estimation coefficient thus achieves our objective: filtering out extreme values and periods of low busy activity, using the remaining throughput data to estimate airport capacity. 




% Real-time capacity is difficult to obtain from historical records directly, which is affected by many factors, including external weather changes and operational factors such as service arrival priority policies or temporary air traffic control. Therefore, based on actual throughput records of arriving and departing flights, we estimate the actual capacity by selecting the most typical time points from the throughput at each 15-minute interval according to defined rules. Specifically, as shown in Equations~\ref{eq: capacity_estimation}, we suppose that the throughput at time $t$ can be represented as 
% \begin{equation}
%     \text{throughput}_t = \min\{\text{demand}_t, \text{capacity}_t\}. 
% \end{equation}
% Thus we have
% \begin{equation}\label{eq: capacity_estimation}
%     \hat{\text{capacity}}_t = \text{throughput}_t \iff  \text{demand}_t \geq \text{throughput}_t + \tau,
% \end{equation}
% where $\tau$ is the integer threshold and $\hat{\text{capacity}}_t$ denotes the estimated capacity at time slice $t$. $\text{throughput}_t$ denotes the throughput at time slice $t$.\par

% We filter the dataset through this definition and control the size of the dataset after estimating capacity using $\tau$. The larger the $\tau$, the smaller the filtered dataset and the more possible estimated capacity. Therefore, selecting an appropriate $\tau$ is a focus. In this study, we obtained five sample datasets by choosing $\tau\in\{1,2,3,4,5\}$. Since each model is trained on a specific airport's dataset, the choice of $\tau$ needs to be based on the parameters of each airport model. The final coefficient is decided as shown in the Table~\ref{tab: coefficient_tau}. Based on these $\tau$ determined separately for each airport's arrival and departure capacity estimates, we filter out time samples when operations are not congested and retain time samples during busy periods, and approximate the real-time capacity to the actual throughput for that time step. However, it is also obvious that using this rule~\ref{eq: capacity_estimation}, capacity is always underestimated as throughput, and busy periods in the evening due to delay propagation are also eliminated. Detailed procedures of coefficient selection is represented in section~\ref{sec: tau_selection}. \par
